# Supplementary material for: Invasion Percolation on Power-Law Branching Processes
Source: arXiv:2208.07827 source file (2023-11-17)
Supplement: Supplementary file 1 [file Supplemental_material.tex]

\section{Supplemental material}

\subsection{Limiting results for \mtitle{$\theta'(p)$} and \mtitle{$\theta^{-1}(p)$}}
\label{app:sec_theta'}

We extend the result of Lemma \ref{lem:deriv_theta} to the  scaling of $\theta'(p)$ around $p=p_c$ and  $\theta^{-1}(x)$ around $x=0$.
We first show that  Lemmas \ref{lem:theta_scaling_>1} and \ref{lem:theta_scaling_<1} extend intuitively to the derivative.
\begin{lemma}[Scaling of the derivative of the survival function]
    Suppose that $\theta(p) = C_\theta  (p-p_c)^{\nu_\alpha}(1+o(1))$. Then
       \begin{equation}
\label{eq:App:theta_deriv_scaling}
    \theta'(p) = C_\theta \nu_\alpha (p-p_c)^{\nu_\alpha-1}(1+o(1)).
\end{equation}
\end{lemma}
\begin{proof}
Starting with $\alpha>2$, the result follows directly from \eqref{eq:implicit_theta'}, as by l'H\^opital's rule
\begin{equation}
\begin{aligned}
\lim_{p\searrow p_c}\theta'(p)&=
    \lim_{p\searrow p_c}
    \frac{\theta(p)\expec[X(1-p\theta(p))^{X-1}]}{1-p\expec[X(1-p\theta(p))^{X-1}]}\\
    &= \lim_{p\searrow p_c}
    \frac{ \theta'(p)\expec[X(1-p\theta(p))^{X-1}] -\theta(p)\expec[X(X-1)(1-p\theta(p))^{X-2}](\theta(p)+p\theta'(p))}{
    p\expec[X(X-1)(1-p\theta(p))^{X-2}](\theta(p)+p\theta'(p))-\expec[X(1-p\theta(p))^{X-1}]}\\&= \lim_{p\searrow p_c}
    \frac{ \theta'(p)\expec[X]}{p_c^2\expec[X(X-1)]\theta'(p) - \expec[X]}(1+o(1)).
\end{aligned}
\end{equation}
Rearranging the terms, gives 
\begin{equation}
    \lim_{p\searrow p_c}\theta'(p) = 
    2\frac{\expec[X]^3}{\expec[X(X-1)]} = C_\theta.
\end{equation}

For the case $\alpha\in(1,2)$, we recall for $p\searrow p_c$,
\begin{equation}
    \expec[X(1-p\theta(p))^{X-1}]
    =
   \Big( \expec[X] -c_{\sss X}(-\Gamma(1-\alpha))\alpha (p\theta(p))^{\alpha-1}\Big)(1+o(1)),
\end{equation}
by \eqref{eq:Bingham_taylor_Derive_alpha(1,2)}.
Substituting this result in \eqref{eq:implicit_theta'} and using the asymptotic behaviour of $\theta(p)$ and the definition of $C_\theta$ of Lemma \ref{lem:theta_scaling_>1}, we find 
\begin{equation}
\begin{aligned}
    \theta'(p) 
    &=
    \frac{ 
    \theta(p) \expec[X(1-p\theta(p)^{X-1}]
    }{-\expec[X](p-p_c)  +\alpha}p^\alpha c_X(-\Gamma(1-\alpha)) C_\theta^{\alpha-1} (p-p_c)
    (1+o(1))
   \\ &= 
    \frac{ C_\theta (p-p_c)^{\frac{1}{\alpha-1}-1}
    \expec[X] }{
    -\expec[X] +\alpha \expec[X]}(1+o(1))
    \\&=
    C_\theta \frac{1}{\alpha-1} (p-p_c)^{\frac{1}{\alpha-1}-1}(1+o(1)).
\end{aligned}    
\end{equation}

For $\alpha\in(0,1)$, 
we again start from \eqref{eq:implicit_theta'}, but now the expectation diverges for $p\searrow p_c$. We recall 
\begin{equation}
    \expec[X(1-p\theta(p))^{X-1}] 
   = \alpha \Gamma(1-\alpha) c_X
    (p\theta(p))^{\alpha-1}(1+o(1)),
\end{equation}
based on \eqref{eq:Bingham_Taylor_theta'_alpha(0,1)}.
Substituting this result in \eqref{eq:implicit_theta'}, we find 
\begin{equation}
\begin{aligned}
    \theta'(p) 
   & = 
    \frac{ C_\theta \alpha\Gamma(1-\alpha)c_X p^{\frac{\alpha}{1-\alpha}}
    }{
    1-p\alpha\Gamma(1-\alpha)c_XC_\theta^{\alpha-1}p^-1
    }(1+o(1))
    \\&=
    \frac{ (c_X\gamma(1-\alpha))^{\frac{\alpha}{1-\alpha}} \alpha c_X\gamma(1-\alpha)}{1-\alpha c_X\gamma(1-\alpha) ( c_X\gamma(1-\alpha))^{-1}}(1+o(1))
    \\&=
    C_\theta \frac{\alpha}{1-\alpha}
    (p-p_c)^{\frac{\alpha}{1-\alpha}-1}(1+o(1)).
\end{aligned}    
\end{equation}
\end{proof}

Finally, we show a convergence result for $\theta^{-1}(x)$ around $x=0$. Similar to $\theta'(p)$, we show that
Lemmas \ref{lem:theta_scaling_>1} and \ref{lem:theta_scaling_<1}
extend intuitively to the inverse:
\begin{lemma}[Scaling of the inverse of the survival function]
    Suppose that $\theta(p) = C_\theta  (p-p_c)^{\nu_\alpha}(1+o(1))$. Then
    \begin{equation}
\label{eq:app:theta_inverse_scaling}
    \lim_{x\searrow 0} \frac{ \theta^{-1}(x) - p_c}{x^{1/\nu_\alpha}} =C_\theta^{-1/\nu_\alpha}.
\end{equation}
\end{lemma}
The result follows from \eqref{eq:App:theta_deriv_scaling}, and there is no distinction between regimes necessary. By l'H\^opital's rule
\begin{equation}
\begin{aligned}
     \lim_{x\searrow 0}\frac{ \theta^{-1}(x) - p_c}{x^{1/\nu_\alpha}}
    &= \lim_{x\searrow 0}
    \frac{ \big[ \theta'(\theta^{-1}(x))\big]^{-1}}{1/\nu_\alpha x^{1/\nu_\alpha-1}}
    \\&=\lim_{x\searrow 0} \frac{ C_\theta^{-1}
    (\theta^{-1}(x) - p_c)^{1-\nu_\alpha}}{
    x^{1/\nu_\alpha-1}}\\&
    =C_\theta ^{-1}\lim_{x\searrow 0}\Big( \frac{
    \theta^{-1}(x) - p_c}{
    x^{1/\nu_\alpha}}\Big)^{1-\nu_\alpha},
\end{aligned}
\end{equation}
where the second equality follows from \eqref{eq:App:theta_deriv_scaling}.
This also implies that 
\begin{equation}
    \lim_{x\searrow 0} \Big(\frac{ \theta^{-1}(x) - p_c}{x^{1/\nu_\alpha}}\Big)^{-\nu_\alpha}= C_\theta,
\end{equation}
from which \eqref{eq:app:theta_inverse_scaling} follows.

\subsection{Bounds on the jump size of \mtitle{$W_k$}}
\label{sec:app:boundjumpsize}
We prove the bounds for the jump size of the $(W_k)_{k\geq0}$ process as presented in \eqref{eq:bounds_jumpsize_alpha(1,2)} and \eqref{eq:couplingbound_alpha<1_2}, for  $\alpha\in(1,2)$ and $\alpha\in(0,1)$ respectively.
Define $\xi_\alpha=\halpha-1$ for $\alpha>2$ or $\alpha\in(1,2)$ and $\xi_\alpha= (1-\alpha)/\alpha$ for $\alpha\in(0,1)$.
Recall also $V_k$ from \eqref{eq:def_V_k} for $\alpha\in(1,2)$ and for simplicity, we take $V_k=W_k$ for $\alpha\in(0,1)$. Then for $x\in[0,1]$ and $k$ large enough, we show that
\begin{equation}
\label{eq:app_jump_bounds}
\underbrace{x^{\xi_\alpha/(1 -\eta_3)} (w_k-p_c)}_{g^{-}(x)} \leq 
    \underbrace{\theta^{-1}(x\theta(W_k))
     -p_c}_{f(x)} \leq  \underbrace{x^{\xi_\alpha/(1+\eta_3)} (w_k-p_c)}_{g^{+}(x)} ,
\end{equation}
which is done in multiple steps. First, we consider $\varepsilon^+>0$ and $\varepsilon^->0$, to be specified later, and show that for some 
large $K$, also specified later, that for all $k>K$
\begin{enumerate}
    \item $g^{-}(0)=f(0)=g^{+}(0)$ and $g^{-}(1)=f(1)=g^{+}(1)$,
    \item $g^{-}(x)\leq f(x)\leq g^{+}(x)$, for $x\in [\varepsilon^-,1-\varepsilon^+]$,
    \item $g^{-}(x)\leq f(x)\leq g^{+}(x)$, for $x\in (0,\varepsilon^-]$,
    \item $g^{-}(x)\leq f(x)\leq g^{+}(x)$, for $x\in [1-\varepsilon^+,1)$.
\end{enumerate}
We consider the above points as the four steps needed to prove \eqref{eq:app_jump_bounds}.
Step 1 follows directly and we therefore focus on showing the other steps below. 
\paragraphi{Step 2} Fix $\varepsilon^->0$ and $\varepsilon^+>0$, where $\varepsilon^{-}$ is formalised in Step 3 and $\varepsilon^{+}$ is formalised in  Step 4. Consider $x\in[\varepsilon^-, 1-\varepsilon^+]$. Then by the approximation in Section \ref{app:sec_theta'}, there exists $u_1,u_2>0$ such that there exists a $K_2(u_1,u_2):=K_2$ such that for all $k>K_2$
\begin{equation}
  (1-u_1) x^{\xi_\alpha} (w_k-p_c) \leq
   \theta^{-1}(x\theta(W_k))
     -p_c \leq  (1+u_2)x^{\xi_\alpha} (w_k-p_c).
\end{equation}
We now choose $1-u_1= x^{\xi_\alpha/(1 -\eta_3)-\xi_\alpha}$ and
$1+u_2= x^{\xi_\alpha/(1 +\eta_3)-\xi_\alpha}$. Under the condition that $x\in[\varepsilon^-, 1-\varepsilon^+]$, we find that 
$0<1-u_1<1$ and $1<1+u_2<C(\varepsilon^-)<\infty$, making the bounds proper. Moreover, as $u_1$ and $u_2$ are uniformly bounded in $\varepsilon^-$ and $\varepsilon^+$, we find that $K_2(u_1,u_2)= K'_2(\varepsilon^-,\varepsilon^+)$.
Substituting the specific choices for $1-u_1$ and $1+u_1$ shows the result. 
\paragraphi{Step 3}
In this step we show that for $x\searrow 0$, $f(x)/g^+(x)\to0$ and $f(x)/g^-(x)\to\infty$, 
which implies that in some small neighbourhood of 0, say $(0,\underline{\varepsilon}]$, that $g^{-}(x)\leq f(x)\leq g^{+}(x)$, 
for $x\in (0,\underline{\varepsilon}]$. This shows the claim, 
and specifies $\varepsilon^-=\underline{\varepsilon}$.
Showing the limits follows intuitively, when we use that, based on \eqref{eq:app:theta_inverse_scaling}, there exists a constant $c$ such that
\begin{equation}
   \lim_{x\searrow 0} \frac{ f(x)}{g^+(x)}=
    \lim_{x\searrow 0}
    \frac{(x\theta(W_k))^{\xi_\alpha} }{x^{\frac{\xi_\alpha}{1+\eta}}(w_k-p_c)}
    \frac{\theta^{-1}(x\theta(W_k))-p_c}{
    (x\theta(W_k))^{\xi_\alpha}}
    = \lim_{x\searrow0}c x^{\xi_\alpha-\frac{\xi_\alpha}{1+\eta}}(1+o(1))=0,
\end{equation}
and
\begin{equation}
   \lim_{x\searrow 0} \frac{ f(x)}{g^-(x)}=
    \lim_{x\searrow 0}
    \frac{(x\theta(W_k))^{\xi_\alpha} }{x^{\frac{\xi_\alpha}{1-\eta}}(w_k-p_c)}
    \frac{\theta^{-1}(x\theta(W_k))-p_c}{
    (x\theta(W_k))^{\xi_\alpha}}
    = \lim_{x\searrow 0}c x^{\xi_\alpha-\frac{\xi_\alpha}{1-\eta}}(1+o(1))=\infty.
\end{equation}

\paragraphi{Step 4} For $x\nearrow 1$, it turns out that it is more convenient to show that for $k$ large enough, to be specified later, $(g^-)'(1) >f'(1) > (g^+)'(1)$. Combined with the result from Step 1 and Step 2, this implies that there exists a small neighbourhood around 1, say $[1-\bar{\varepsilon},1)$, such that for all $x\in[1-\bar{\varepsilon},1)$,
 $g^{-}(x)\leq f(x)\leq g^{+}(x)$. This shows the claim and specifies $\varepsilon^+=\bar{\varepsilon}$.
 
 We next find the derivatives 
 \begin{equation}
 \begin{aligned}
      f'(1) = \frac{d}{dx}\Big[ \theta^{-1}(x\theta(W_k))\Big]_{x=1}
      =\Big[\frac{\theta(W_k)}{\theta'(\theta^{-1}(x\theta(W_k))}\Big]_{x=1} =\frac{\theta(W_k)}{\theta'(W_k)},
 \end{aligned}
 \end{equation}
 and 
 \begin{equation}
     (g^\pm)'(1) = \Big[ \frac{\xi_\alpha}{1\pm\eta} x^{\frac{\xi_\alpha}{1\pm\eta}-1} (W_k-p_c)\Big]_{x=1} = \frac{\xi_\alpha}{1\pm\eta}(W_k-p_c).
 \end{equation}
 In order to compare $f'(1)$ and $(g^\pm)'(1)$, we use Lemmas \ref{lem:theta_scaling_>1} and \ref{lem:theta_scaling_<1} and \eqref{eq:App:theta_deriv_scaling} to simplify $f'(1)$. Specifically, there exists a $K_4^+(\eta):=K_4^+$, such that for all $k>K_4^+$
 \begin{equation}
    f'(1) = \frac{\theta(W_k)}{\theta'(W_k)}
    > \frac{1}{1+\eta} 
    \frac{ C_\theta(W_k-p_c)^{1/\xi_\alpha} }{
    1/\xi_\alpha C_\theta(W_k-p_c)^{1/\xi_\alpha-1}}
    =\frac{\xi_\alpha}{1+\eta} (W_k-p_c)
    .
 \end{equation}
 Similarly, there exists a $K_4^-(\eta):=K_4^-$, such that for all $k>K_4^-$
 \begin{equation}
    f'(1) = \frac{\theta(W_k)}{\theta'(W_k)}
    < \frac{1}{1-\eta} 
    \frac{ C_\theta(W_k-p_c)^{1/\xi_\alpha} }{
    1/\xi_\alpha C_\theta(W_k-p_c)^{1/\xi_\alpha-1}}
     =\frac{\xi_\alpha}{1-\eta} (W_k-p_c)
     .
 \end{equation}
 Combining this with $g'(1)$, this directly implies, for $k>\max\{K_4^+,K_4^-\}$
 \begin{equation}
     \frac{f'(1)}{(g^+)(1)'} >1,
     \quad 
     \text{ and } 
     \quad 
     \frac{f'(1)}{(g^-)(1)'} <1.
 \end{equation}
 This shows the claim.
 
 \paragraphi{Combining the results}
 Step 1 through Step 4 show that  $g^-(x)<f(x)<g^+(x)$ for $x\in[0,1]$ with the specified choices of $\varepsilon$ and $k$ large enough. Indeed, for given $\eta$ small, say $\eta<1/2$ to avoid trivial cases, we find that Step 3 determines an $\varepsilon^-$ and step 4 determines an $\varepsilon^+$. 
 With the fixed values of $\varepsilon^+$ and $\varepsilon^-$, Step 2 determines $K'_2$ and Step 4 determines $ K_4^+$ and $K_4^-$, so that for the result holds for all $k>\max\{K'_2,K_4^+,K_4^-\}$.

\subsection{Mass functions and tail distributions}
\label{sec:app_mass_tail}
We show how one can write a sum of mass function to the tail distribution. It is straightforward to verify that, for an arbitrary function $f(x)$ and a discrete random variable $X$ defined on the integers and for $a\geq 0$,  
\begin{equation}
\label{eq:app_mass_tail_lem1}
    \sum_{i> a} f(i) \prob(X=i)
    =
    f(a) \prob(X>a-1)+ \sum_{i>a } \Big( f(i+1)-f(i)\Big)\prob(X>i).
\end{equation}

\begin{comment}
\begin{proof}
We compute
\begin{equation}
 \begin{aligned}
 \sum_{i> a} f(i) \prob(X=i)&=
  \sum_{i> a} f(i) (\prob(X>i-1)-\prob(X>i))\\
  &=  f(a) \prob(X>a-1)
 + \sum_{i> a+1} f(i)\prob(X>i-1)
  -\sum_{i> a} f(i) \prob(X>i)\\
  &=  
  f(a) \prob(X>a-1)
 + \sum_{i> a} f(i+1)\prob(X>i)
  -\sum_{i> a} f(i) \prob(X>i)\\
   &= f(a) \prob(X>a-1)
 + \sum_{i> a} \Big(f(i+1)-f(i)\Big)\prob(X>i).
 \end{aligned}
 \end{equation}
\end{proof}
\end{comment}
We show how the result of \eqref{eq:app_mass_tail_lem1} can be used to derive explicit scaling result for specific tail distribution. In the specific case where $w_k=p_c(1+a/k)$ we also notice that $\theta(w_k)$ converges to 0 uniformly in $a\in[\varepsilon,1/\varepsilon]$. Therefore, the errors small in $\theta(w_k)\searrow0$, are also  uniformly small in $a$ on bounded intervals, which we recall from \eqref{eq:small-o}, as $\o{k}{a}$.

\begin{lemma}
\label{lem:app_mass_tail_lem2}
Let $\alpha$ be given, then for $m\in{1,2}$
\begin{equation}
     \sum_{i>x/\hat{\theta}(w_k)} i^m(1-\hat{\theta}(w_k))^{i-1} 
    \prob(X=i)= \frac{\alpha c_{\sss X}}{\hat\theta(w_k)^{m-\alpha}}\int_x^\infty \e^{-z} z^{m-1-\alpha} \dif z(1+\o{k}{a}).
\end{equation}
\end{lemma}

\begin{proof}
We first apply the result of \eqref{eq:app_mass_tail_lem1} with $a=x/\hat\theta(w_k)$ and $f(x)=x(1-\hat\theta(w_k))^{x-1}$, which implies
\begin{equation}
\label{eq:Dbk_alpha<1_auxeq_1}
\begin{aligned}
     \sum_{i>x/\hat{\theta}(w_k)}&
     i^m(1-\hat{\theta}(w_k))^{i-1} 
    \prob(X=i) =
   \Big( \frac{x}{\hat\theta(w_k)}
   \Big)^{m}
   (1-\hat\theta(w_k))^{x/{\hat\theta(w_k)}-1}\Big(\frac{x}{\theta(w_k)}-1\Big)^{-\alpha}
    \\&+
    \sum_{i>x/\hat{\theta}(w_k)}
    [-i^m\hat\theta(w_k)+ 2i^{m-1}(m-1)+1] 
    (1-\hat\theta(w_k))^{i-1}
    \prob(X>i)(1+\o{k}{a}),
\end{aligned}
\end{equation}
where we use that $1-\hat\theta(w_k))=1+\o{k}{a}.$
Let us focus on the first term in the sum first, where we can see that it splits in two parts. 
As $1/\hat\theta(w_k)$ diverges for $k\to\infty$, the tail of the sum can be properly approximated by an integral, we find for the first part
\begin{equation}
\begin{aligned}
\label{eq:Dbk_alpha<1_auxeq_2}
   &- \hat\theta(w_k)\sum_{i>x/\hat{\theta}(w_k)}( 
    (1-\hat\theta(w_k))^{i-1}c_{\sss X} i^{m-\alpha}
   \\&\qquad  =-\hat\theta(w_k)\int_{x/\hat\theta(w_k)}^\infty 
    (1-\hat\theta(w_k))^{i-1}c_{\sss X} i^{m-\alpha} \dif i(1+\o{k}{a}).
    \end{aligned}
\end{equation}
We substitute $z= -i\log(1-\hat\theta(w_k))$ and Taylor expand it since for $k\to\infty$. Also, by partial integration  \eqref{eq:Dbk_alpha<1_auxeq_2} simplifies to 
\begin{equation}
\begin{aligned}
\label{eq:Dbk_alpha<1_auxeq_3}
    &-\frac{\hat\theta(w_k)c_{\sss X}}{[\hat\theta(w_k)
    +O(\hat\theta(w_k)^2)]^{m+1-\alpha}
    }
    \int_x^\infty \e^{-z} z^{m-\alpha} \dif z(1+\o{k}{a})
    \\&\qquad = -\frac{c_{\sss X}}{\hat\theta(w_k)^{m-\alpha}}
    \Big[
    x^{m-\alpha}\e^{-x} + (m-\alpha)  \int_x^\infty \e^{-z} z^{m-\alpha-1} \dif z 
    \Big] (1+\o{k}{a}).
    \end{aligned}
\end{equation}
We can apply a similar argument for the second part to show that 

\begin{equation}
\begin{aligned}
\label{eq:Dbk_alpha<1_auxeq_12}
    & 2(m-1)c_{\sss X} \sum_{i>x/\hat{\theta}(w_k)}  
   (1-\hat\theta(w_k))^{i-1}i^{m-\alpha-1}
 \\&\qquad  = 
     2(m-1) \frac{c_{\sss X}}{\hat\theta(w_k)^{m-\alpha}}
   \int_{x}^\infty 
   \e^{-z}z^{m-\alpha-1}\dif z(1+\o{k}{a}).
   \end{aligned}
\end{equation}

Finally, for the third part
\begin{equation}
\label{eq:Dbk_alpha<1_auxeq_4}
     \sum_{i>x/\hat{\theta}(w_k)}( 
    (1-\hat\theta(w_k))^{i}c_{\sss X} i^{-\alpha}
    =
    c_{\sss X}\hat\theta(w_k)^{\alpha-1}
    \int_x^\infty \e^{-z} z^{-\alpha} \dif z(1+\o{k}{a}).
\end{equation}
By filling in the results of \eqref{eq:Dbk_alpha<1_auxeq_3} and \eqref{eq:Dbk_alpha<1_auxeq_4} in \eqref{eq:Dbk_alpha<1_auxeq_1}, it follows that the numerator in \eqref{eq:Dbk_alpha<1_auxeq_0} simplifies for the case $m=1$ to 
\begin{equation}
\begin{aligned}
    &
    c_{\sss X}\hat{\theta}(w_k)^{-(1-\alpha)}
    \Big[
    x^{1-\alpha} \e^{-x}
-    
    (
    x^{-\alpha+1}\e^{-x} + (-\alpha)  \int_x^\infty \e^{-z} z^{-\alpha} \dif z )\Big] (1+\o{k}{a}) \\
    &= \alpha c_{\sss X}\hat\theta(w_k)^{-(1-\alpha)}\int_x^\infty \e^{-z} z^{-\alpha} \dif z (1+\o{k}{a}).
    \end{aligned}
\end{equation}
By similar reasoning, filling in the results of \eqref{eq:Dbk_alpha<1_auxeq_3} ,\eqref{eq:Dbk_alpha<1_auxeq_12} and \eqref{eq:Dbk_alpha<1_auxeq_4} in \eqref{eq:Dbk_alpha<1_auxeq_1}, it follows that the numerator in \eqref{eq:Dbk_alpha<1_auxeq_0} simplifies for the case $m=2$ to 
\begin{equation}
     \frac{c_{\sss X} \alpha}{\hat\theta^{2-\alpha}(w_k) } 
   \int_x^\infty \e^{-z}z^{1-\alpha} \dif z (1+\o{k}{a}).
\end{equation}

\end{proof}

\subsection{Uniform convergence in \mtitle{$a$}}
\label{app:sec_uniform_conv}
In Section~\ref{sec-size-trees-off-backbone-alpha>2} in Equations \eqref{eq:54_uniformly_in_a} and \eqref{Bin-LCLT-cons-a3} we argue convergence of the process is uniform in $a$ on bounded intervals. In most cases this follows trivially, but here we show that 
\begin{equation}
\label{eq:uniform_a_eq1}
    \frac{ 
    (n- (Q_n+D_{v_k^\star} )w_k)^2}
    {n(1-w_k)}
    \xrightarrow{d}
    \frac{(\sigma p_c Z+a\sqrt{x})^2}{1-p_c}.
\end{equation}
uniformly in $a$ on bounded intervals, where $Z\sim \mathcal{N}(0,1)$. Recall that here it is assumed that $w_k=p_c(1+a/k)$ and note that the left-hand side of \eqref{eq:uniform_a_eq1} can be rewritten as 
\begin{equation}
\label{eq:uniform_a_eq2}
    \bigg[
    \frac{n\mu - Q_n}{\mu\sqrt{n(1-w_k)}}
    +\frac{ Q_n a p_c}{k\sqrt{n(1-w_k)}}
    +\frac{D_{v_k^\star}w_k }{\sqrt{n(1-w_k)}}
    \bigg]^2,
\end{equation}
For the first part, we see clearly that 
\begin{equation}
        \frac{n\mu - Q_n}{\mu\sqrt{n(1-w_k)}}
    \xrightarrow{d}
     \frac{\sigma}{\mu\sqrt{1-p_c}}\mathcal{N}(0,1),
\end{equation}
uniformly in $a$, as for $a\in[\varepsilon,1/\varepsilon]$ the only term that has an $a$ is given by $w_k=p_c(1-a/k)\leq p_c(1-\varepsilon/k)\to 0 $. 
Furthermore, the limiting random variable is normally distributed which has a continuous CDF, which implies absolute uniform continuity with respect to the Lebesgue measure.
According to the same reason we can write 
\begin{equation}
    \frac{ Q_n a}{k\sqrt{n(1-w_k)}}
    \xrightarrow{\prob}
    \frac{\sqrt{x} a}{\sqrt{1-p_c}},
\end{equation}
uniformly in $a$ on bounded intervals and 
\begin{equation}
    \frac{D_{v_k}^\star w_k }{\sqrt{n(1-w_k)}}
    \xrightarrow{\prob} 
    0,
\end{equation}
uniformly in $a$ on bounded intervals. 
Combining these results, by uniform Slutzky's theorem \cite[Theorem 6.3]{Bengs2019}, we find
\begin{equation}
    \frac{n\mu - Q_n}{\mu\sqrt{n(1-w_k)}}
    +\frac{ Q_n a p_c}{k\sqrt{n(1-w_k)}}
    +\frac{D_{v_k^\star}w_k }{\sqrt{n(1-w_k)}}
    \xrightarrow{d}
    \frac{\sigma p_c}{\sqrt{1-p_c}}Z
    +
      \frac{\sqrt{x} a}{\sqrt{1-p_c}},
\end{equation}
uniformly in $a$. The right hand side still admits a continuous CDF and by the uniform continuous mapping theorem \cite[Theorem 6.2]{Bengs2019}, \eqref{eq:uniform_a_eq1} follows uniformly in $a$ on bounded intervals.
\begin{comment}
\begin{equation}
    \bigg(\frac{n\mu - Q_n}{\mu\sqrt{n(1-w_k)}}
    +\frac{ Q_n a p_c}{k\sqrt{n(1-w_k)}}
    +\frac{D_{v_k^\star}w_k }{\sqrt{n(1-w_k)}}\bigg)^2
    \xrightarrow{d} \bigg( 
    \frac{\sigma p_c}{\sqrt{1-p_c}}\mathcal{N}(0,1)
    +
     \frac{\sqrt{x} a}{\sqrt{1-p_c}} \bigg)^2,
\end{equation}
uniformly in $a$. 
\end{comment}
Again, we see  that the right-hand side admits a continuous CDF. Then, by the uniform equivalence theorem for continuously bounded $f$
\cite[Corollary 4.2]{Bengs2019}, this then implies
\begin{equation}
\begin{aligned}
    &\expec\bigg[ f\bigg( \Big(\frac{n\mu - Q_n}{\mu\sqrt{n(1-w_k)}}
    +\frac{ Q_n a p_c}{k\sqrt{n(1-w_k)}}
    +\frac{D_{v_k^\star}w_k }{\sqrt{n(1-w_k)}}\Big)^2\bigg)\bigg]
    \\&\qquad\to
   \expec\bigg[f
    \bigg( \Big(\frac{\sigma p_c}{\sqrt{1-p_c}}Z
    +
     \frac{\sqrt{x} a}{\sqrt{1-p_c}} \Big)^2\bigg)\bigg],
     \end{aligned}
\end{equation}
uniform in $a\in[\varepsilon,1/\varepsilon]$.

\subsection{Proof of the local limit theorem of \mtitle{$\alpha$}-stable random variables for \mtitle{$\alpha\in(1,2)$}}
\label{app:sec_local_lims_upper_bound_mass_alpha(1,2)}
Let $\tilde X^{\sss(k)}_i$ have the distribution as given in \eqref{eq:def_tilde_X}, then we show that $\sup_\ell\prob(\tilde X^{\sss(k)}_1 + \cdots+\tilde X^{\sss(k)}_n = \ell) \leq Cn^{1/\alpha}$ for some fixed $C$ and $\alpha\in(1,2)$. 
\begin{proof}[Proof of Lemma~\ref{lem:local_lims_upper_bound_mass_alpha(1,2)}]
Fix $\alpha\in(1,2)$.
Let us assume for convenience that the random variables are of mean 0. Otherwise one can subtract $n$ times the mean from both sides.
 Let $\phi_k(u)$ denote the characteristic function of $\tilde X^{\sss(k)}$ then we use inverse transforms to find the general bound
 \begin{equation}
     \sup_\ell 
     \prob(\tilde X^{\sss(k)}_1+\cdots+\tilde X^{\sss(k)}_n= \ell) =
     \sup_\ell 
     \frac{1}{2\pi} \int_{-\pi}^{\pi}
     \e^{-i u\ell} \phi_k(u)^n\dif u
     \leq 
     \frac{1}{2\pi} \int_{-\pi}^{\pi} 
     |\phi_k(u)|^n\dif u.
 \end{equation}
 We next show that the integral scales as $n^{-1/\alpha}$.
 The proof is split in two parts, where we make a distinction between different integral regimes. There, we need to show the following two properties:
 \begin{enumerate}
     \item[(a)] For some $\delta>0$ small enough, there exists some $C$ such that for $|u|<\delta$
     \begin{equation}
     \label{eq:massfuncbound_a}
         |\phi_k(u)|< 1- C|u|^{\alpha}. 
     \end{equation}
     \item[(b)] For this same $\delta$, there exists some $\varepsilon>0$ such that for $|u|\geq\delta$
     \begin{equation}
     \label{eq:massfuncbound_b}
         |\phi_k(u)| < 1-\varepsilon.
     \end{equation}
 \end{enumerate}
 We first show that under conditions (a) and (b) the proof follows, after which we prove the conditions in more detail.
 
 Suppose that (a) and (b) are true, then there exists some $\delta,\varepsilon>0$ and a fixed constant $C$ such that
 \begin{equation}
 \begin{aligned}
     \frac{1}{2\pi} 
     \int_{-\pi}^\pi 
     |\phi_k(u)|^n\dif u 
    & \leq 
     \frac{1}{2\pi}\int_{-\delta}^\delta 
     (1-|u|^\alpha)^n \dif u 
     +C(1-\varepsilon)^n \\&
     \leq
 \frac{2}{2\pi}\int_{0}^{\delta} \e^{-nu^\alpha}\dif u+ C(1-\varepsilon)^n.
\end{aligned}
 \end{equation}
 By a substitution from $nu^\alpha=x$ and noting that $-1+1/\alpha>- 1$, gives
 \begin{equation}
 \begin{aligned}
   \frac{1}{\pi}\int_{0}^{\delta} \e^{-nu^\alpha}\dif u &\leq
 \frac{1/\alpha-1}{\pi}n^{-1/\alpha} \int_{0}^{n\delta^\alpha} \e^{-x} x^{-1+1/\alpha}\dif x(1+o(1))
 \\&
 \leq \frac{1/\alpha-1}{\pi}n^{-1/\alpha}\int_0^\infty \e^{-x}x^{1/\alpha-1}\dif x(1+o(1))
 \\&=
  C n^{-1/\alpha}(1+o(1)).
  \end{aligned}
\end{equation}
 We continue by showing (a) and (b).
 
 We start with (a) and show that \eqref{eq:massfuncbound_a} holds.
 Recall that the distribution of $\tilde X^{\sss(k)}$ can also be written as $\prob(\tilde X^{\sss(k)} = \ell) = \eta(w_k)^\ell 
 \prob(\Binom(X,w_k)=\ell)$. Therefore, we also find for the characteristic function of $\tilde X^{\sss(k)}$
 \begin{equation}
     \phi_k(u) = \eta(w_k)^{-1} \expec[(1- (1-\e^{ui}\eta(w_k))w_k)^X].
 \end{equation}
We expand the characteristic function of $X$, which follows a power-law distribution with exponent $\alpha\in(1,2)$. Based on \cite[Theorem 8.1.6]{Bingham1987}, we find by taking $w_k=p_c(1+a/k)$
 \begin{equation}
 \begin{aligned}
  \phi_k(u)& =
    \eta(w_k)^{-1} \Big(
     1 -\expec[X] (-\log(1-w_k(1-\e^{i u}\eta(w_k))))\\
  &\quad   +c_{\sss X}(-\Gamma(1-\alpha)) (-\log(1-w_k(1-\e^{i u}\eta(w_k))))^\alpha
     \Big)(1+\o{k,1/u}{a}).
     \end{aligned}
 \end{equation}
 Expanding the logarithmic term results in 
 \begin{equation}
  \label{eq:app_bound_CF_1}
 \begin{aligned}
  \phi_k(u) &=  \eta(w_k)^{-1}\Big(
     1-\expec[X](w_k(1-\e^{i u} \eta(w_k)))\\&\quad
     +c_{\sss X}(-\Gamma(1-\alpha))w_k^\alpha(1-\e^{iu}\eta(w_k)))^\alpha  \Big)(1+\o{k,1/u}{a})\\&
     =
     \Big(a/k+\e^{iu}(1+a/k)
      +\eta(w_k)^{-1}c_{\sss X}(-\Gamma(1-\alpha))w_k^\alpha(1-\e^{iu}\eta(w_k))^\alpha\Big)(1+\o{k,1/u}{a}).
    \end{aligned}
 \end{equation}
 Here, the error term is small in for $k$ large and $u$ small. Next, we take absolute values on both sides, where we use
 \begin{equation}
 \label{eq:Janson_eqaulity_fixed}
    \log( |\phi_k(u) | )
     =\log\Big( \Big| \e^{Re( \log(\phi_k(u))) + i Im(\log(\phi(u)))}\Big|\Big)
     = \log\Big( \Big| \e^{Re( \log(\phi_k(u)))}\Big|\Big)
     =Re(\log(\phi_k(u)))
     .
 \end{equation}
 Furthermore, we note that in our regime $k$ is generally large and consider that case specifically. Therefore, there exists a $K$ such that for all $k>K$, $w_k$ and $\eta(w_k)$ are uniformly bounded in $a\in[\varepsilon,1/\varepsilon]$. By \eqref{eq:Janson_eqaulity_fixed} 
 \begin{equation}
     \begin{aligned}
     |\phi_k(u)|&\leq 
     \exp\Big\{ Re\Big[ \log\Big(
     \Big(
     \e^{iu}
      +C(1-\e^{iu}\eta(w_k))^\alpha\Big) (1+\o{k,1/u}{a})\Big)\Big]
     \Big\}\\&=
     \exp\Big\{Re\Big[ \log\Big(1-(1- \e^{iu})+ C(1-\e^{iu}\eta(w_k))^\alpha\Big)\Big]\Big\}
     (1+\o{k,1/u}{a})\\
     &= 
      \exp\Big\{Re\Big[-(1- \e^{iu})+ C(1-\e^{iu}\eta(w_k))^\alpha\Big]\Big\}
      (1+\o{k,1/u}{a}).
\end{aligned}
\end{equation}
We bound this expression by noting that $Re(1-\e^{iu})\geq 0$ and $\eta(w_k)^{\alpha}<1$, so that uniformly in $k$
\begin{equation} 
\begin{aligned}
    |\phi_k(u)|  &\leq 
      \exp\Big\{\eta(w_k)^{\alpha}CRe\Big[ (1-\e^{ui})^\alpha
      \Big]\Big\}(1+\o{k,1/u}{a})\\
&=
      \exp\{C^{*} |u|^\alpha 
      Re( (-i)^\alpha) 
      \}(1+\o{k,1/u}{a}).\\
     \end{aligned}
 \end{equation}
 Note that $(-i)^\alpha = \exp( -\alpha\pi/4)\in (-1,0)$ for $\alpha \in(1,2)$. Therefore there exists a $c$ such that $Re(i^\alpha)=-c.$ This concludes that for $u$ small enough, say smaller than some specific $\delta>0$, that
 \begin{equation}
 \label{eq:app:Janson_result_1}
     |\phi_k(u)| \leq \e^{-c|u|^\alpha}
     =(1-C|u|^\alpha)(1+\o{k,1/u}{a})
     .
 \end{equation}
 Next, we consider (b) and show that  \eqref{eq:massfuncbound_b} holds uniformly for $k>K^*$, where $K^*<\infty$ is large enough as will be specified later. Define 
 \begin{equation}
     \label{eq:def_phi_app}
     \phi(u) = \lim_{k\to\infty} \phi_k(u)
     =
     \expec[ (1-(1-\e^{iu})p_c)^X],
 \end{equation}
 then by the triangle inequality we can bound for $u\in[-\pi,\pi]\setminus(-\delta,\delta)$
 \begin{equation}
     |\phi_k(u)|
     \leq |\phi_k(u)- \phi(u)| + |\phi(u)|.
 \end{equation}
 %In the following we show that for the specified region for $u$,
 %$|\phi_k(u)-\phi(u)|<\varepsilon$ for all $k>K^*$ and 
 %$|\phi(u)|<1-2\varepsilon$, which then shows the claim in \eqref{eq:massfuncbound_b}.\\
 Firstly, $\phi_k(u)\to \phi(u)$, and as $\phi_k(u)$ is a characteristic function $\tilde X^{\sss(k)}$, which converges in distribution to $X$, by the continuity theorem \cite[Section 14.7, Theorem 15]{Fristedt1997}, convergence of the characteristic function follows and is uniform on $u\in [-\pi,\pi]$. Therefore, for a given $\varepsilon>0$, there exists a finite $K^*$ such that for all $k>K^*$ $|\phi_k(u)-\phi(u)|<\varepsilon$, uniformly in $u$ on $[-\pi,\pi]$.\\
 Secondly
 \begin{equation}
     |\phi(u)|\leq \expec[ \e^{X\log | 1-(1-\e^{-ui})p_c|}].
 \end{equation}
By \eqref{eq:Janson_eqaulity_fixed}, we can restrict ourselves to the real part in the logarithm to obtain
\begin{equation}
\begin{aligned}
    \expec[ \e^{X\log | 1-(1-\e^{-ui})p_c|}]
    =&
     \expec[ \e^{X Re\{ \log(1-(1-\e^{-ui})p_c)}\}]
     =\expec[ \e^{X Re\{ -(1-\e^{iu})p_c - O((1-\e^{iu})^2p_c^2) 
     \}}]\\
     &\leq\expec[\e^{-p_cX(1-\cos(u))} \e^{-Xp_c|(1-\e^{ui})^2p_c^2|}]
     \\&\leq  \expec[\e^{-p_cX(1-\cos(u))}].
    \end{aligned}
\end{equation}
For $|u|>\delta$, we see that $\cos(u)<1$, so that for some given $\varepsilon$, there exists a $\delta>0$, such that for $|u|>\delta$ and $|u|\leq\pi$, 
\begin{equation}
    |\phi(u)| < 1-2\varepsilon.
\end{equation}
 Combining this with the first step shows \eqref{eq:massfuncbound_b}.
\end{proof}
